# Supplementary material for: Robust Vision-Based Runway Detection through Conformal Prediction and Conformal mAP
Source: arXiv:2505.16740 source file (2025-05-22)
Supplement: Supplementary file 1 [file map.tex]

\begin{algorithm}[H]
\caption{Pseudo-code for mAP Calculation}
\label{alg:map}
\begin{algorithmic}[1]
\STATE \textbf{Input:} 
\STATE \quad A set of predicted bounding boxes \(\{(B_i, o_i, p_i)\}_i\) for each class
\STATE \quad A set of ground truth bounding boxes \(\{(B^{gt}_j, c_j)\}_j\) for each class
\STATE \quad IoU threshold range \([0.5, 0.95]\)
\STATE \quad Step size for IoU threshold: \(\Delta t = 0.05\)
\STATE \textbf{Output:} mAP score

\FOR{each class \( c_k \)}
    \STATE Initialize precision and recall lists: \(\text{Precision}(c_k)\), \(\text{Recall}(c_k)\)
    \FOR{each IoU threshold \( t \) in \([0.5, 0.55, 0.6, \dots, 0.95]\)}
        \STATE Initialize true positives \( \text{TP}(t) \), false positives \( \text{FP}(t) \), and false negatives \( \text{FN}(t) \)
        \FOR{each predicted bounding box \( (B_i, o_i, p_i) \)}
            \STATE Find the best matching ground truth box \( B^{gt}_j \) based on IoU
            \IF{IoU between \( B_i \) and \( B^{gt}_j \) is greater than or equal to \( t \)}
                \STATE Increment \( \text{TP}(t) \) (True Positive)
            \ELSE
                \STATE Increment \( \text{FP}(t) \) (False Positive)
            \ENDIF
        \ENDFOR
        \FOR{each ground truth box \( (B^{gt}_j, c_j) \)}
            \IF{No matching prediction for \( B^{gt}_j \)}
                \STATE Increment \( \text{FN}(t) \) (False Negative)
            \ENDIF
        \ENDFOR
        \STATE Calculate precision and recall at threshold \( t \):
        \[
        \text{Precision}(t) = \frac{\text{TP}(t)}{\text{TP}(t) + \text{FP}(t)}
        \]
        \[
        \text{Recall}(t) = \frac{\text{TP}(t)}{\text{TP}(t) + \text{FN}(t)}
        \]
        \STATE Store the precision-recall values at this IoU threshold for plotting
    \ENDFOR

    \STATE Plot the precision-recall curve for class \( c_k \)
    \STATE Compute the area under the precision-recall curve (AP) for class \( c_k \)
    \STATE Store the AP value for class \( c_k \)
\ENDFOR

\STATE \textbf{Output:} 
\STATE Calculate the mean average precision (mAP) across all classes:
\[
\text{mAP} = \frac{1}{C} \sum_{k=1}^{C} \text{AP}(c_k)
\]
\STATE Return the mAP score
\end{algorithmic}
\end{algorithm}
