# Supplementary material for: Robust Vision-Based Runway Detection through Conformal Prediction and Conformal mAP
Source: arXiv:2505.16740 source file (2025-05-22)
Supplement: Supplementary file 2 [file model.tex]

\section{Hyperparameters}
\label{appendix:data_augmentation}

\begin{table}[h]
\centering
\begin{tabular}{|l|c|p{8cm}|}
\hline
\textbf{Augmentation} & \textbf{Value} & \textbf{Description} \\
\hline
\texttt{hsv\_h} & 0.015 & Hue augmentation factor applied to images for color variation. \\
\texttt{hsv\_s} & 0.7 & Saturation augmentation factor to modify color intensity. \\
\texttt{hsv\_v} & 0.4 & Value (brightness) augmentation factor to adjust image lightness. \\
\texttt{degrees} & 0.0 & Rotation range in degrees for random image rotation. \\
\texttt{translate} & 0.1 & Fraction of total image size used for random translations. \\
\texttt{scale} & 0.5 & Scaling factor to zoom in or out of the image. \\
\texttt{shear} & 0.0 & Shear intensity for distortion along the image axes. \\
\texttt{flipud} & 0.0 & Probability of vertical flip (up-down). \\
\texttt{fliplr} & 0.5 & Probability of horizontal flip (left-right). \\
\texttt{mosaic} & 1.0 & Probability of applying mosaic augmentation (combines 4 images). \\
\texttt{mixup} & 0.0 & Probability of applying mixup augmentation (blends 2 images). \\
\texttt{copy\_paste} & 0.0 & Probability of copy-pasting objects between images. \\
\hline
\end{tabular}
\caption{YOLOv5 data augmentation settings and their descriptions.}
\label{tab:yolov5_augmentation}
\end{table}
